# Supplementary material for: Fermionic UV models for neutral triple gauge boson vertices
Source: arXiv:2402.04306 source file (2024-11-25)
Supplement: Supplementary file 1 [file appendix.tex]

\appendix

\section{Additional material}
